# Supplementary material for: When to Accept Automated Predictions and When to Defer to Human Judgment?
Source: arXiv:2407.07821 source file (2024-08-13)
Supplement: Supplementary file 1 [file 07-Appendix-original.tex]

\clearpage
\appendix
\section{Appendix}
\label{appendix:supplemtary-material}

\subsection{Plots}
Figure \ref{fig:cifar10_combined_confusion_matrix} shows the confusion matrix for CIFAR-10 training and testing data ViT predictions. Noticeable on the training dataset is the spread of misclassifications, where the highest is between cat and dog (182) and dog and cat  (174) classes, and the lowest (0) is between frog and truck. In the training dataset, the most misclassified class is dog (33) and the least  is frog (0).
Conversely in Figure \ref{fig:CIFAR10_testing_plot_accuracy_decrements} in can be observed that class cat and dog are the classes that the ViT model predicts least accurately, and a threshold decrement to 10\% of the original threshold would still provide confidence that nearly 95\% of predictions are 100\% accurate, while for the frog class, were the threshold to be set at 10\% of the original threshold, would still provide confidence that over 98\% of predictions below threshold and 100\% accurate.
The overall plot on the right of Figure \ref{fig:CIFAR10_testing_plot_accuracy_decrements}, shows that if the threshold were to be set at 10\% of the original threshold for all classes, 97.5\% of predictions would be below threshold, and considered 100\% accurate, while 2.25\% of the class predictions would be defered.

% plot produced with function call:
% conf_matrix1, conf_matrix2 = display_misclassifications_side_by_side_cifar10(train_np, test_np, 10, 11, class_labels, 20, 7, True)
\begin{figure}[h]
    \centering   
    \includegraphics[width=0.99\columnwidth]{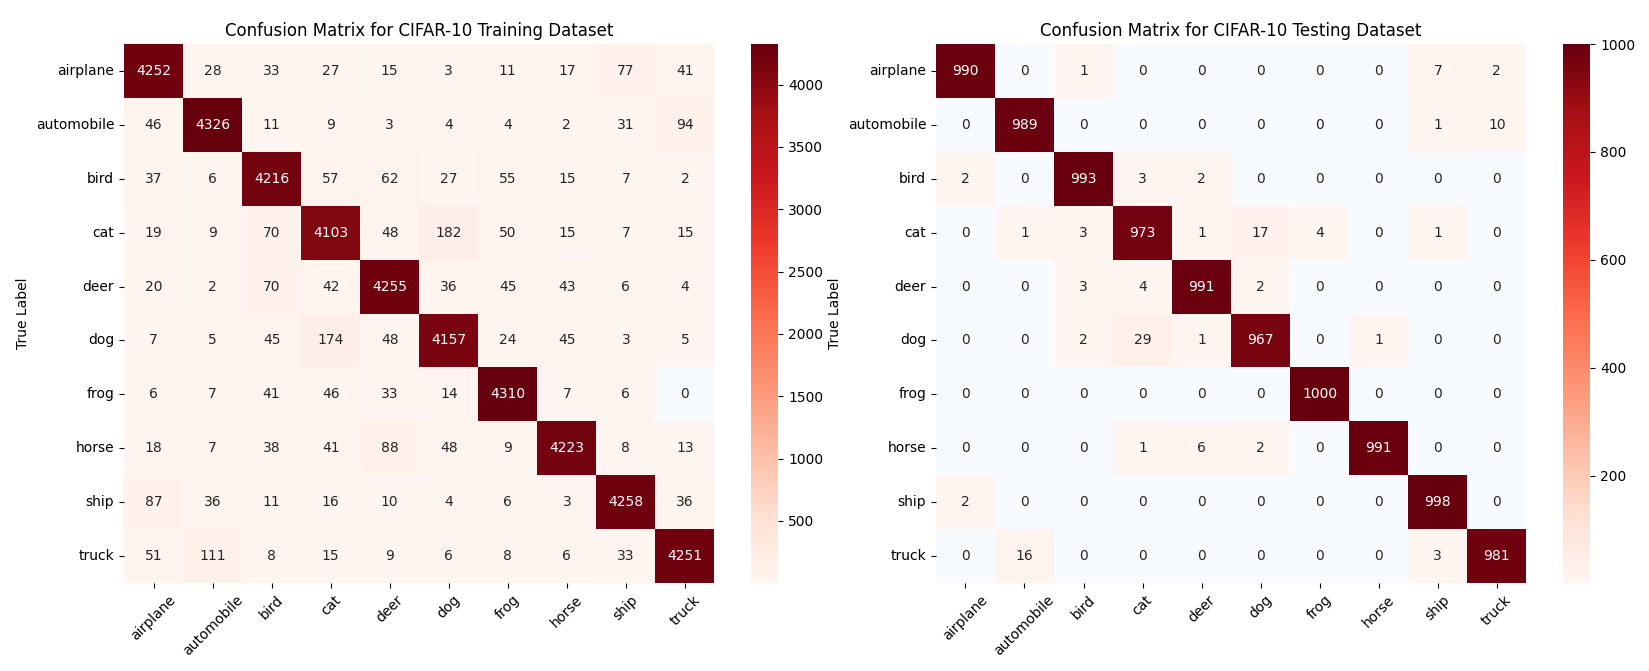}
    \caption{Please zoom in for detail. Confusion matrices for the CIFAR-10 classification model on the training dataset (left) and testing dataset (right). The matrices display the true labels on the vertical axis and the predicted labels on the horizontal axis. The diagonal elements represent correctly classified instances, while the off-diagonal elements indicate misclassifications.}
    \label{fig:cifar10_combined_confusion_matrix}
\end{figure}

%%%%%%%%%%%%%%%%%%%%%%%%%%%%%%%%%%%%%%%%%%%%%%%%%%%%
% PLOT ALL TESTING DATASET CLASS ACCURACY DECREMENTS %
%%%%%%%%%%%%%%%%%%%%%%%%%%%%%%%%%%%%%%%%%%%%%%%%%%%%%%

% Plot generated with function call
% plot_accuracy_decrements(accuracy_results, 
                         % overall_results,
                         % labels=class_labels, 
                         % save=True, 
                         % x_label='Threshold Decrement Factor', 
                         % title='CIFAR10 Testing Dataset Class Prediction Accuracy vs Distance to Threshold Decrement Factor', 
                         % filename='CIFAR10_testing_plot_accuracy_decrements.png')

\begin{figure}[h]
    \centering
\includegraphics[width=0.99\columnwidth]{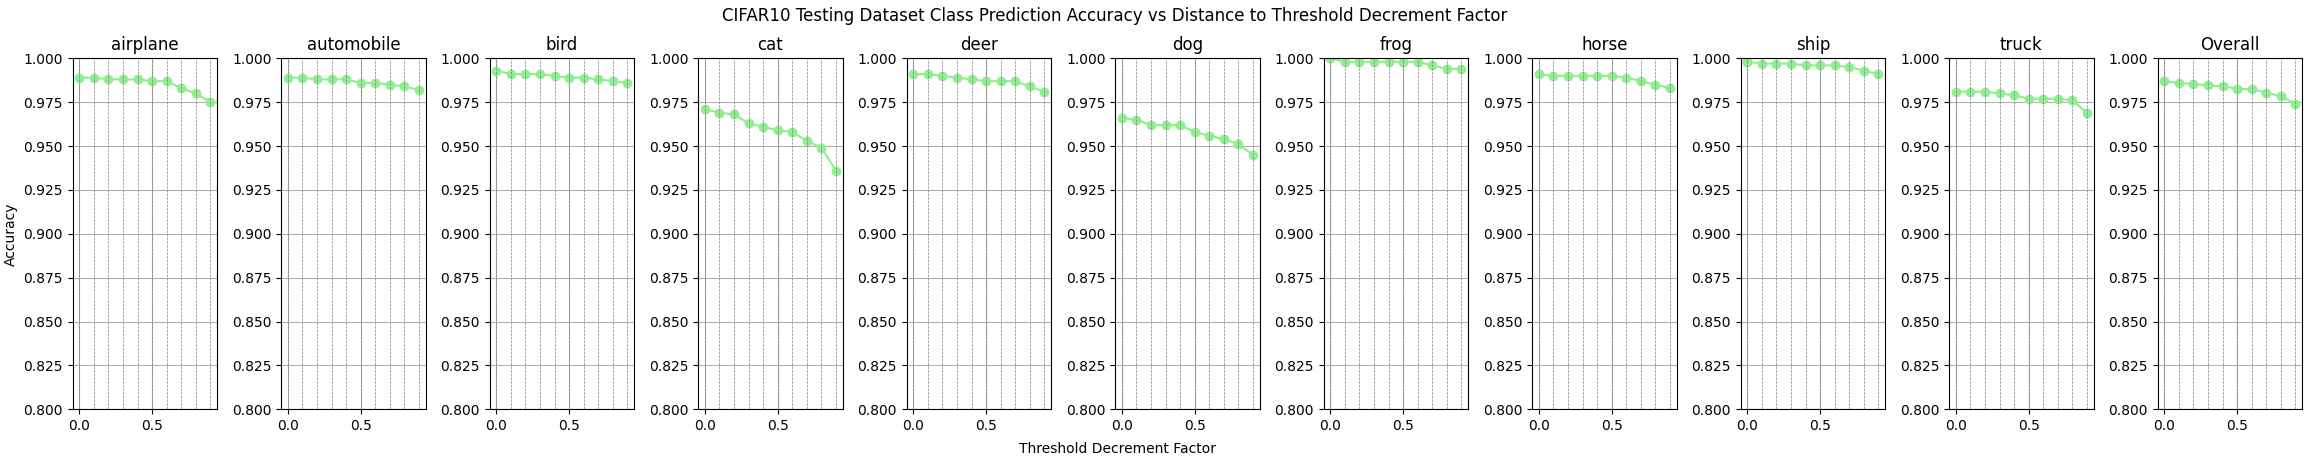}
    \caption{Please zoom in for detail. Accuracy decrements for CIFAR-10 testing data in threshold decrease factors of 0.1}
    \label{fig:CIFAR10_testing_plot_accuracy_decrements}
\end{figure}

Figure \ref{fig:CIFAR10_testing_plot_accuracy_decrements} shows the expected accuracy decrement for the CIFAR-10 training dataset as the threshold decreases in factors of 0.1.

% \begin{figure}[h]
%     \centering    
%     \includegraphics[width=0.99\columnwidth]{Figures/CIFAR10_single_plot_accuracy_decrements.png}
%     \caption{Single plot Accuracy decrements}   \label{fig:CIFAR10_single_plot_accuracy_decrements}
% \end{figure}

% The accuracy on the training dataset in 98.38\% and 98.46\% on the testing dataset. Figure \ref{fig:mnist_combined_misclassifications}. 

\begin{figure}[h]
    \centering
    \includegraphics[width=0.99\columnwidth]{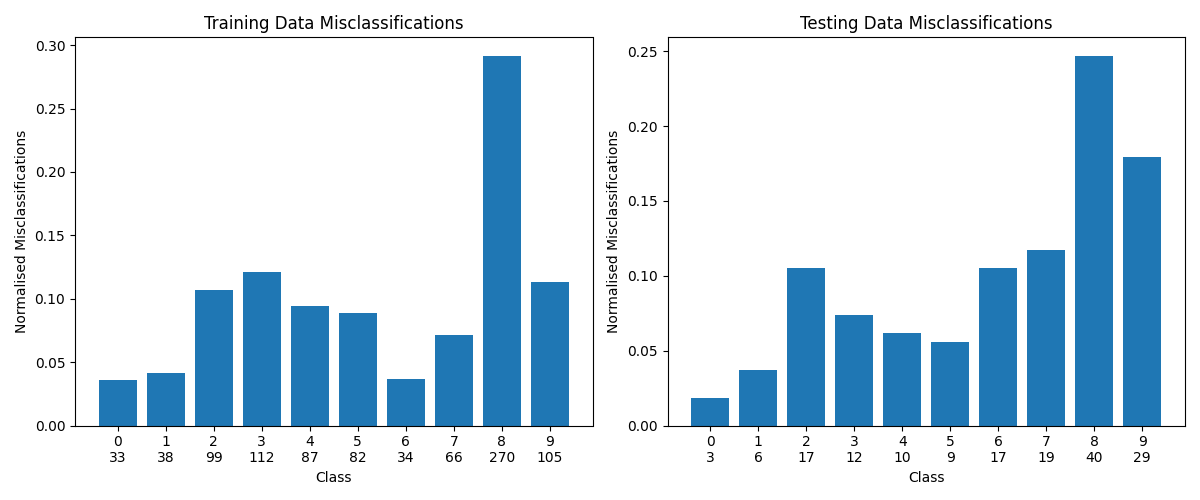}
    \caption{Normalised misclassifications for each class in the training data (left) and testing data (right). The x-axis represents the class labels from 0 to 9, with the corresponding non-normalised misclassification count displayed below each label. The y-axis shows the normalized misclassifications, obtained by dividing the misclassification count for each class by the total number of misclassifications in the respective dataset. }
    \label{fig:mnist_combined_misclassifications}
\end{figure}


Our k-means cluster for 59074 correct MNIST digit predictions converges in a fraction of a second. We then plot the mean distance to centroids for every class in Figure \ref{fig:MNIST_Correct_Training_and_Testing_Mean_Distance_To_Centroids}.

\begin{figure}[h]
    \centering
    \includegraphics[width=0.99\columnwidth]{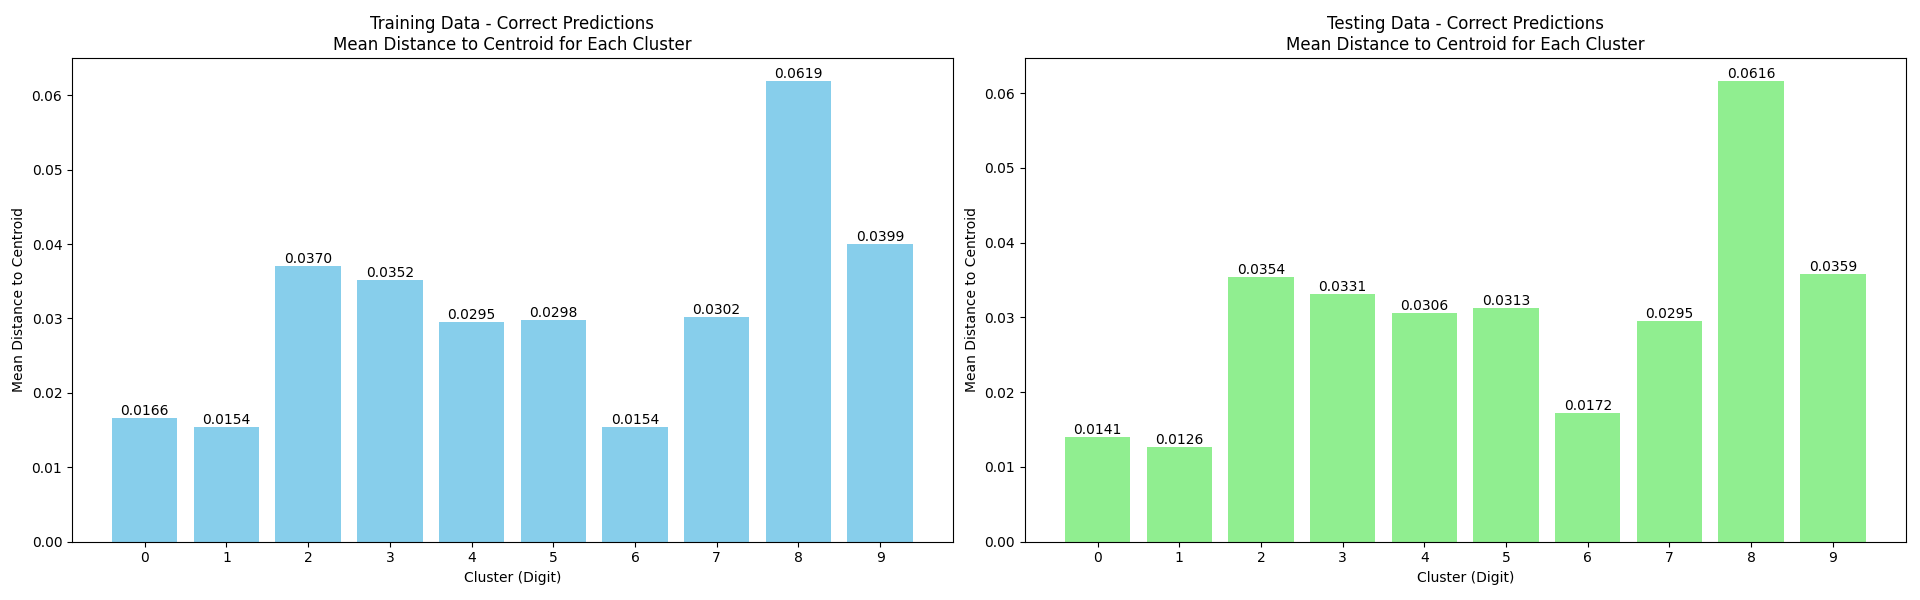}
    \caption{Mean distances for Softmax function output for each class, for correct classifications. On the right is the plot for the training dataset and the corresponding test dataset on the right.}
    \label{fig:MNIST_Correct_Training_and_Testing_Mean_Distance_To_Centroids}
\end{figure}

% Accuracy decrements

Figure \ref{fig:plot_accuracy_decrements} refers to the MNIST dataset and shows accuracy on y axis and decrement in factors of 0.1 e.g. at 0.1 the threshold would be 90\% distant from centroid compared to threshold (minimum distance to centroid from all misclassifications for the class). Noticeable is digit 8, that presents the highest number of misclassifications in both training and testing datasets, and the steepest drop in accuracy as a result of the threshold becoming closer to the centroid. Also noticeable are digits that the network predicts with high accuracy, e.g. 1 and 2, still would present relatively high accuracy even if the threshold was to be placed at 10\% of the original threshold. 
\begin{figure}[h]
    \centering
\includegraphics[width=0.99\columnwidth]{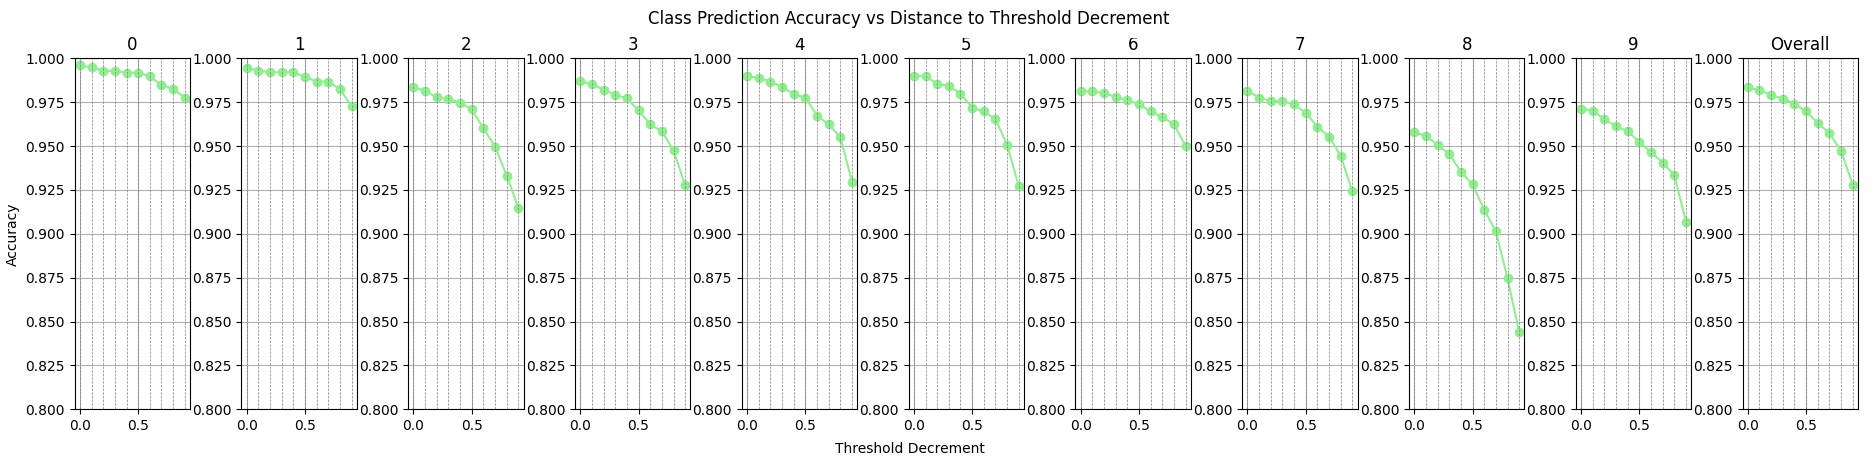}
    \caption{Zoom in for detail. Accuracy decrements}
    \label{fig:plot_accuracy_decrements}
\end{figure}

Figure \ref{fig:plot_accuracy_decrements}

The boxplots in Figure \ref{fig:boxplots_side_by_side_x2_training_centroids} compare the distribution of distances to centroids for correctly and incorrectly classified instances across different digit classes in both the training and testing MNIST datasets. In the testing dataset (right plot), by referencing as a reminder Table 

In the training data (left plot), the distances for correctly classified instances are lower than those of incorrectly classified instances across all digit classes. This indicates that the distance of the Softmax output to the K-Means cluster centroids are good candidate proxies for accuracy, leading to smaller distances for correct classifications.
%%%%%%%%%%%%%%%%%%%%%%%%%%%%%%%%%%%%%%%%%%%%%%%%%%%%%%%%%%%%%%%
% Average Softmax Probabilities for Correctly and Incorrectly %
% Classified Classes in the CIFAR10 dataset                   %
%%%%%%%%%%%%%%%%%%%%%%%%%%%%%%%%%%%%%%%%%%%%%%%%%%%%%%%%%%%%%%%

% Plot generated by function call
% single_plot_accuracy_decrements(accuracy_results, overall_results, labels=class_labels, dataset="CIFAR10", save=True)

% \begin{figure}[h]
%     \centering    
%     \includegraphics[width=0.99\columnwidth]{Figures/CIFAR10_single_plot_accuracy_decrements.png}
%     \caption{Single plot Accuracy decrements}   \label{fig:CIFAR10_single_plot_accuracy_decrements}
% \end{figure}

% Function call to generate plot
% plot_centroid_distance_bars(train_correct_predictions, 
                            % train_incorrect_predictions, 
                            % labels=class_labels, 
                            % color1='lightblue', 
                            % color2='lightcoral', 
                            % data="CIFAR10 Training Data", 
                            % save=True, 
                            % filename='CIFAR10_training_plot_centroid_distance_bars.png')


\begin{figure}[h]
    \centering
    \includegraphics[width=0.95\columnwidth]{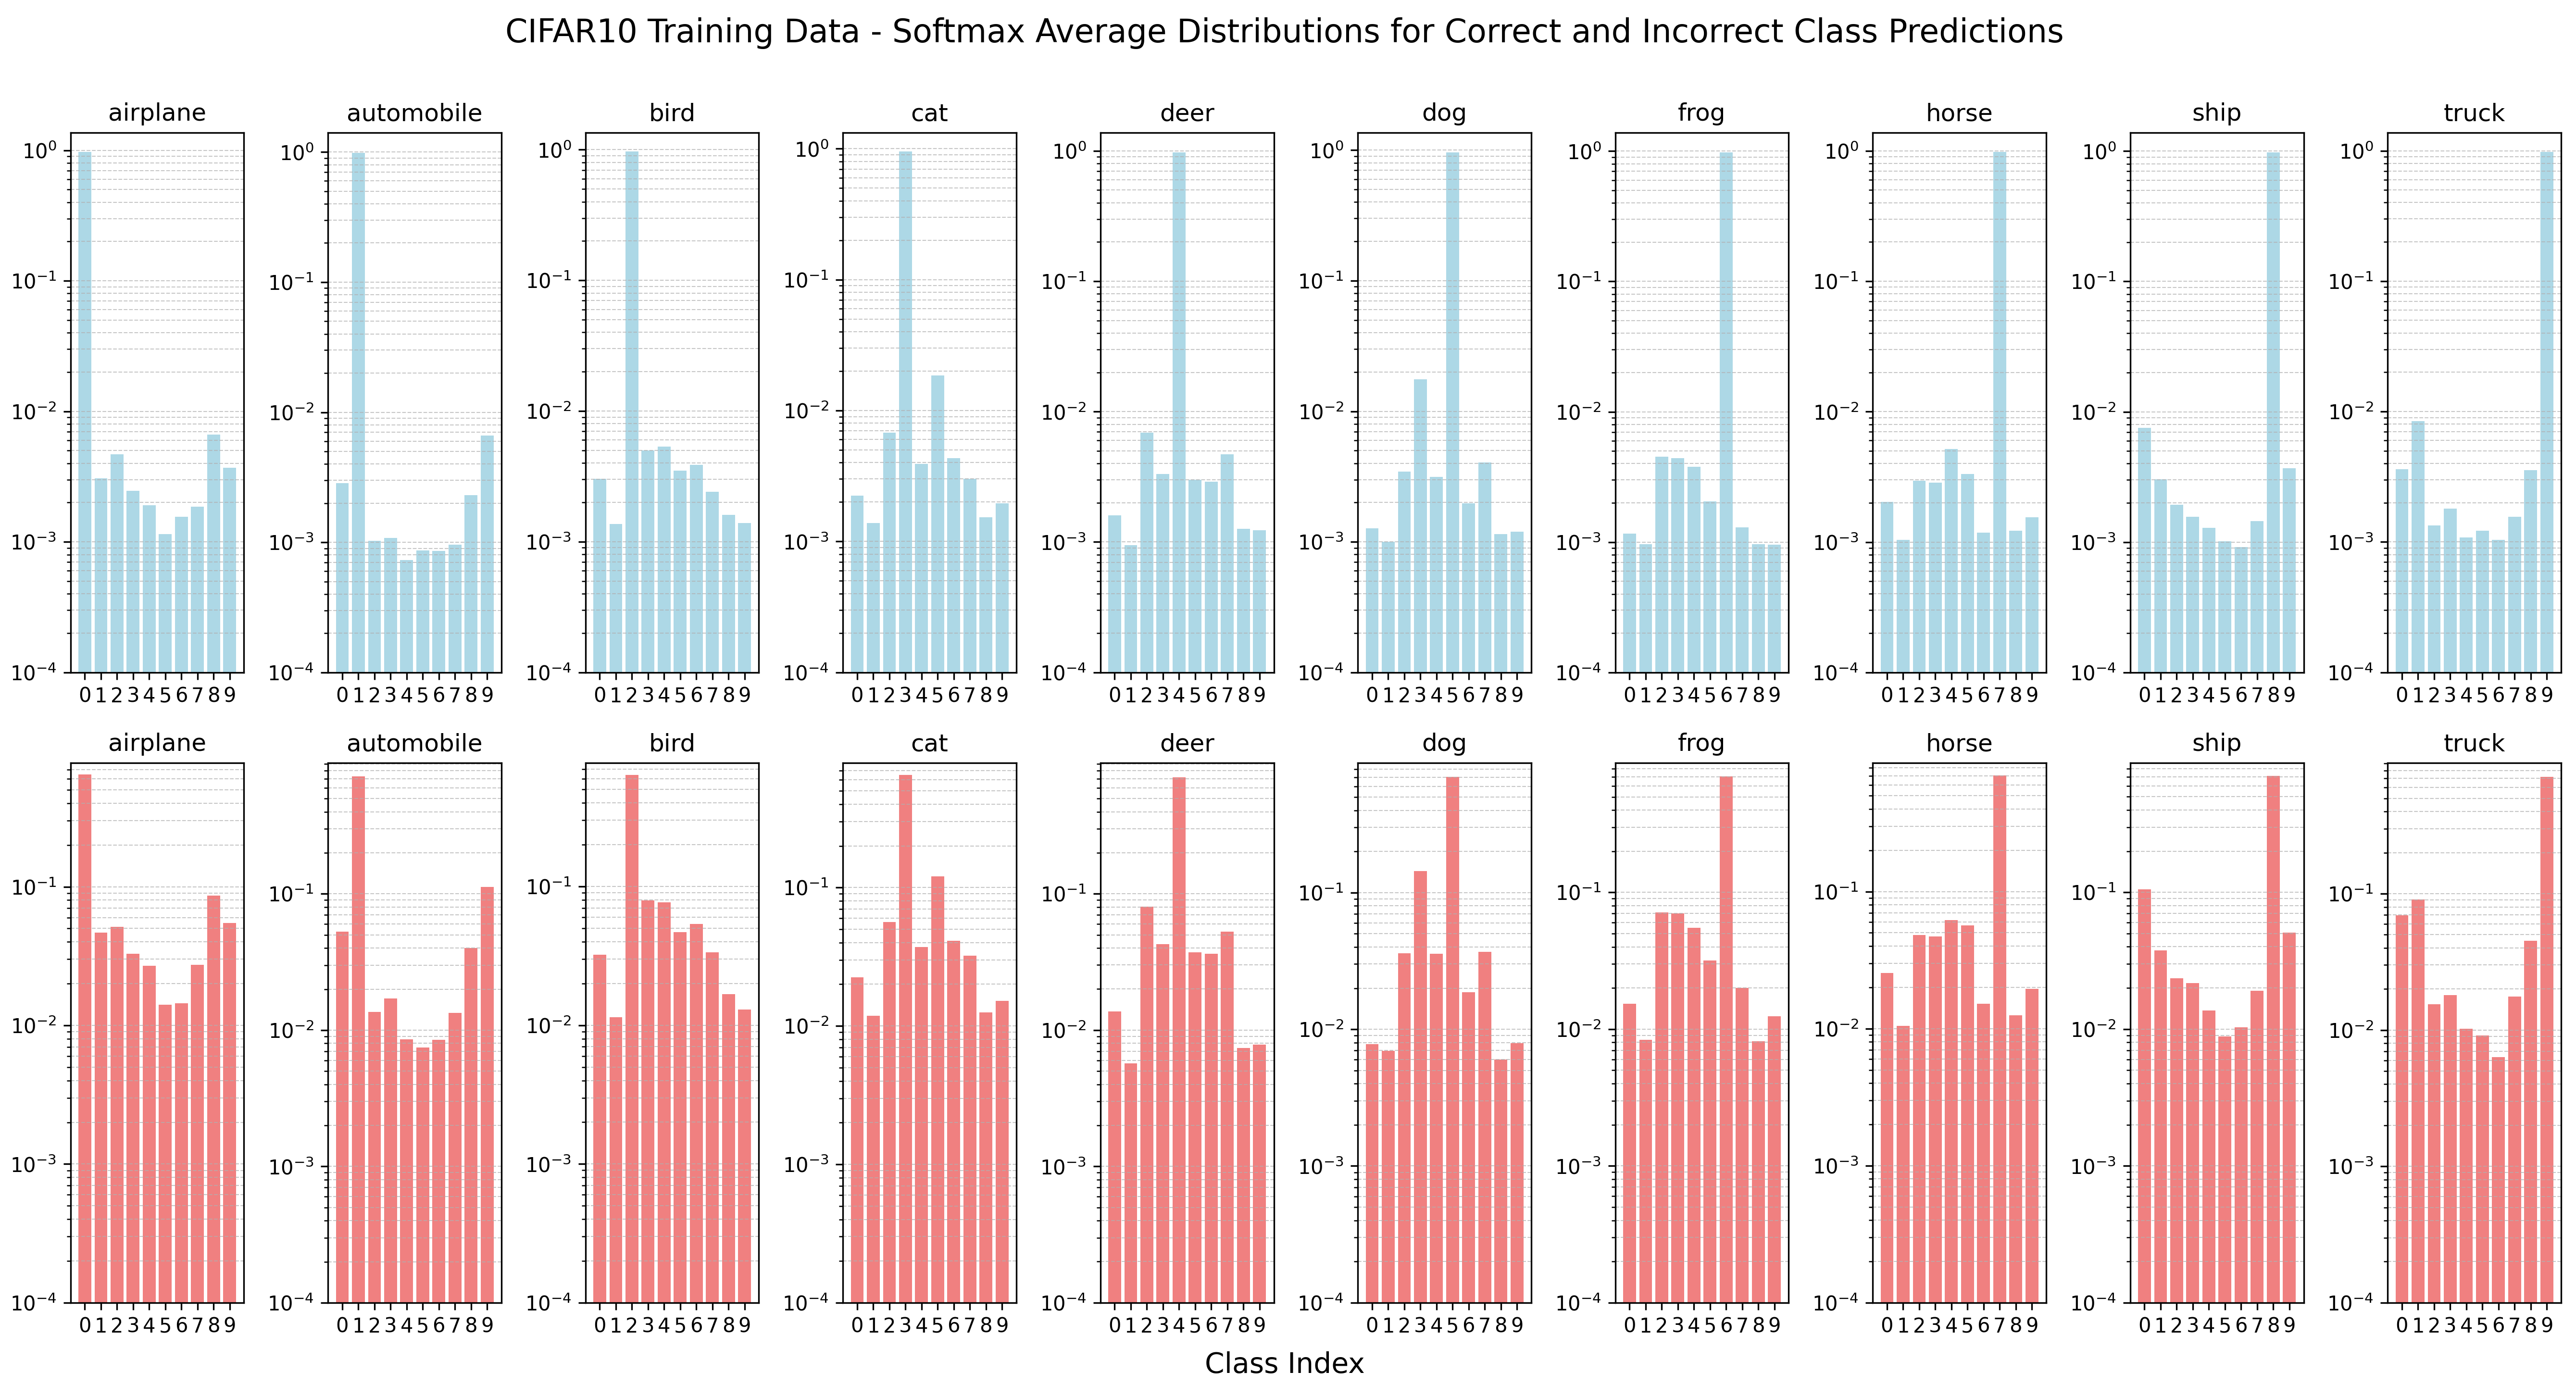}
    \caption{Please zoom in for detail. Average Softmax Probabilities for Correctly and Incorrectly Classified Classes in the CIFAR-10 Training Dataset}
    \label{fig:CIFAR10_training_plot_centroid_distance_bars.png}
\end{figure}

% Function call to generate plot
% plot_centroid_distance_bars(test_correct_predictions, 
%                             test_incorrect_predictions, 
%                             labels=class_labels, 
%                             color1='lightgreen', 
%                             color2='lightcoral', 
%                             data="CIFAR10 Testing Data", 
%                             save=True, 
%                             filename='CIFAR10_testing_plot_centroid_distance_bars.png')

\begin{figure}[h]
    \centering
    \includegraphics[width=0.95\columnwidth]{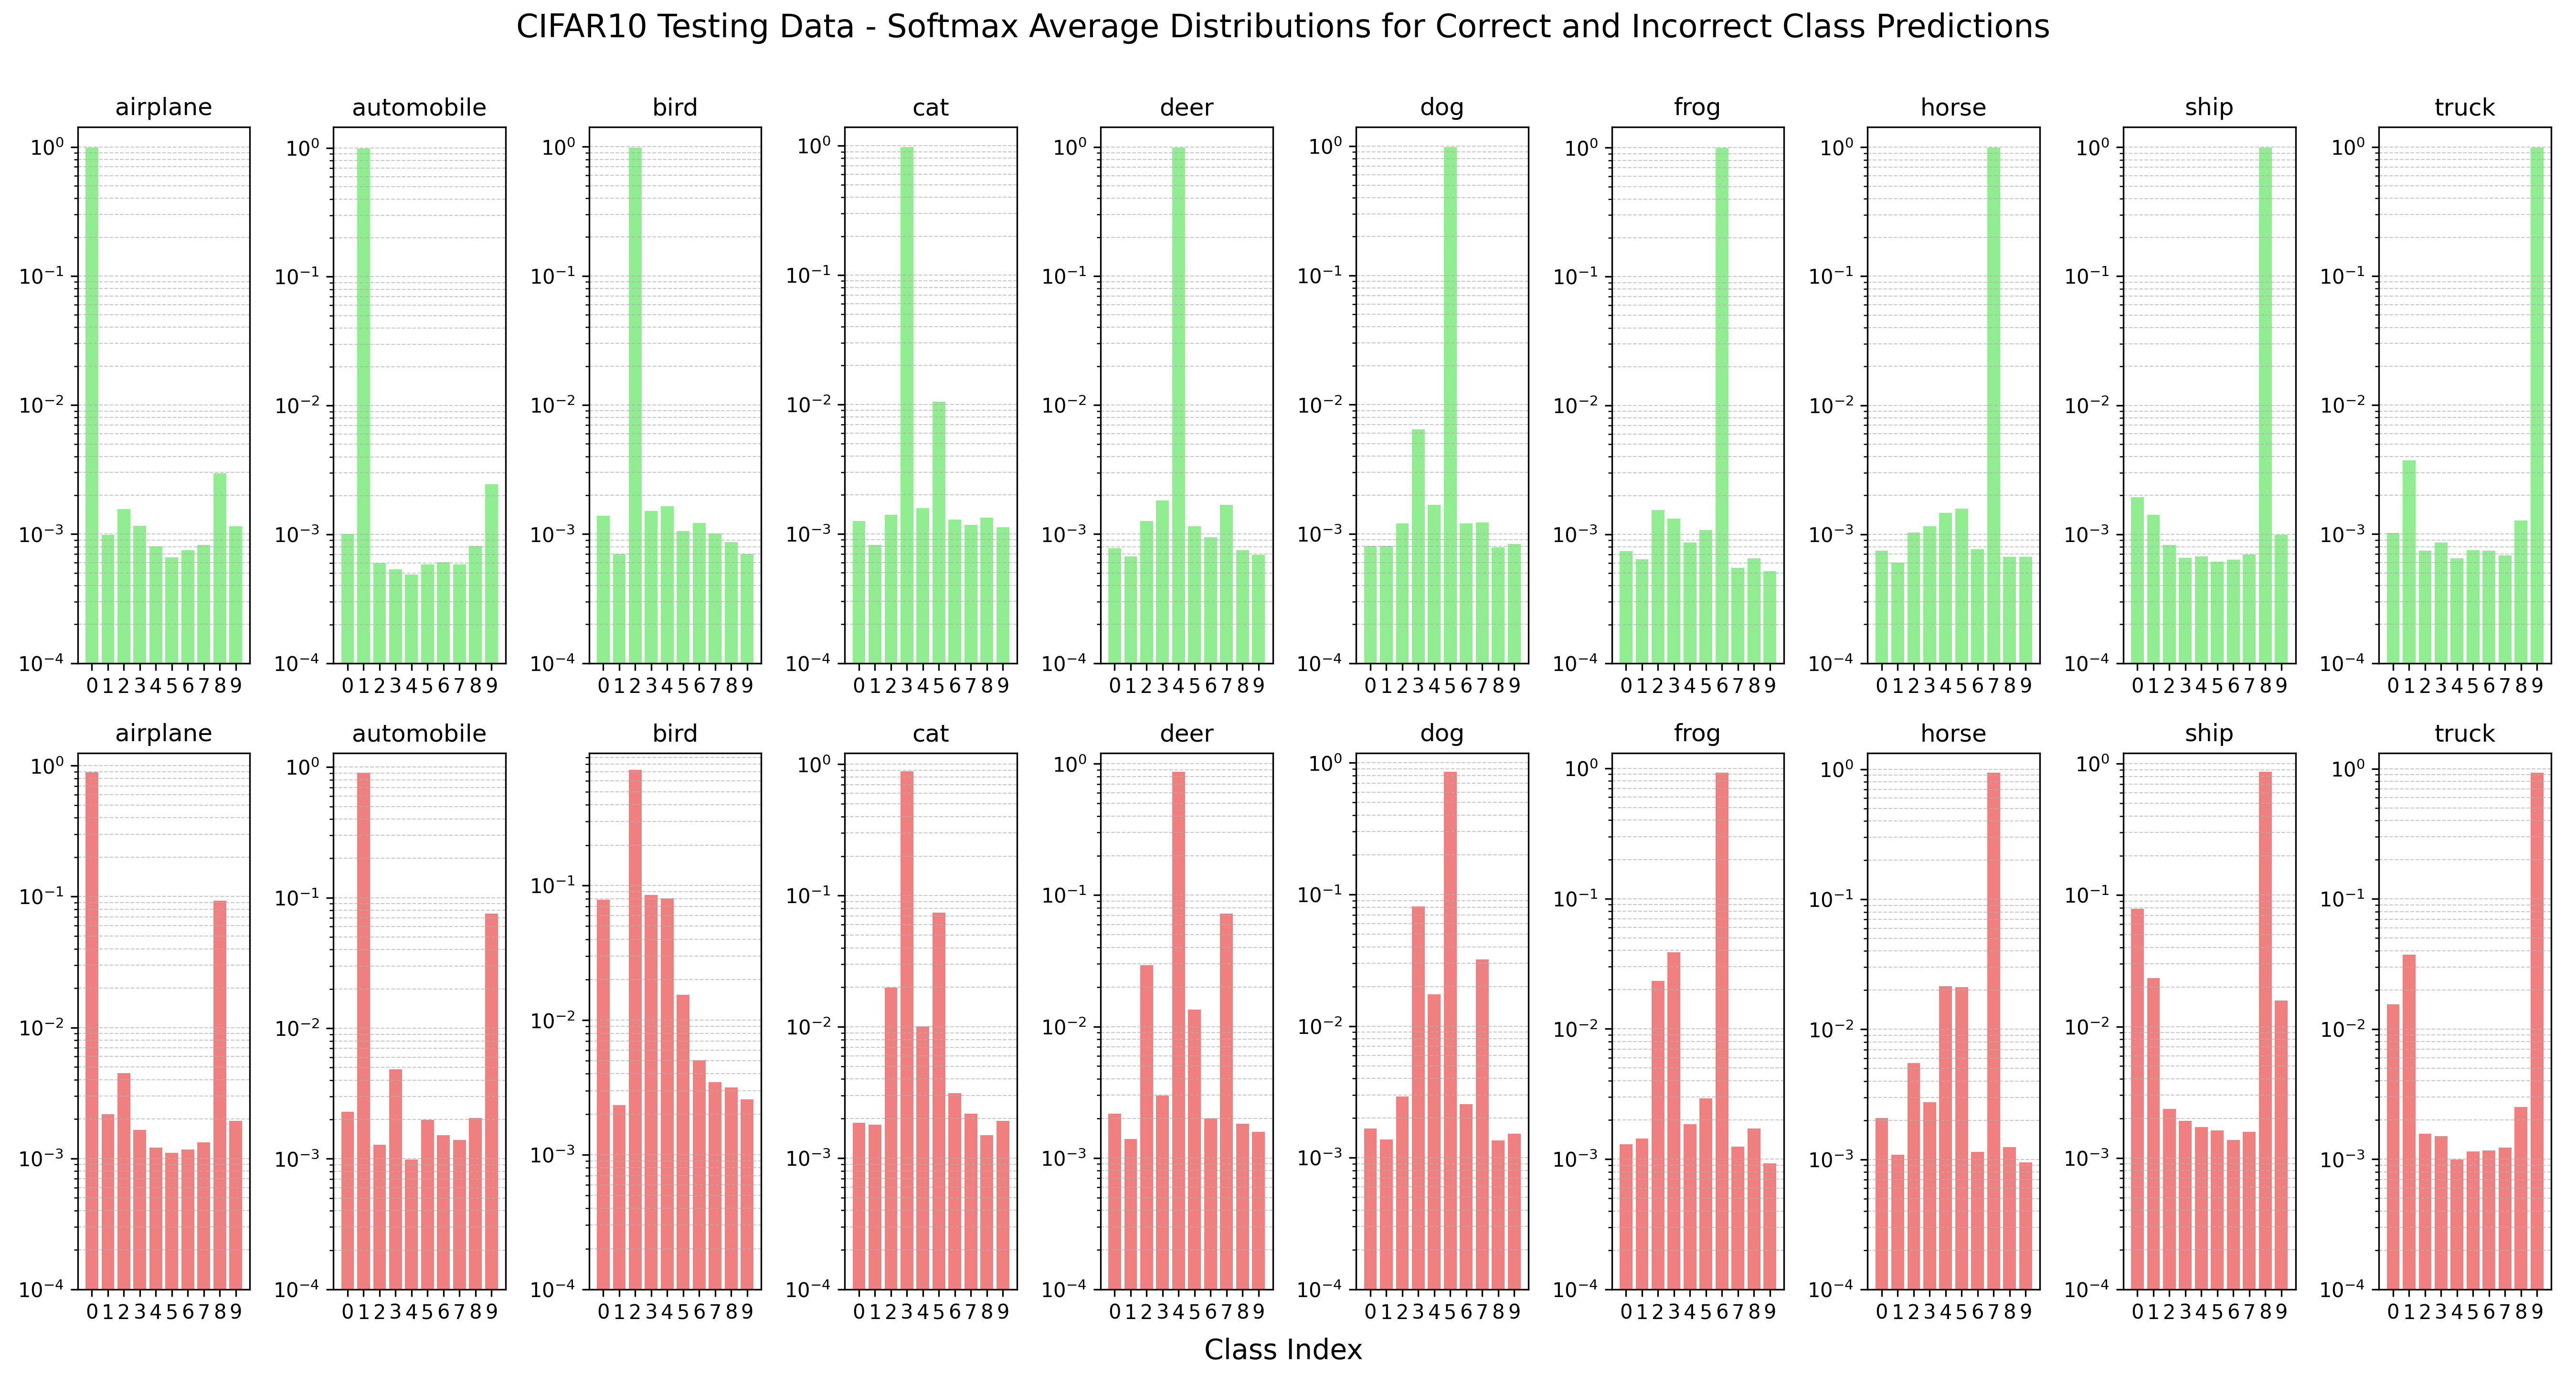}
    \caption{Please zoom in for detail. Average Softmax Probabilities for Correctly and Incorrectly Classified classes in the CIFAR-10 Testing Dataset}
    \label{fig:CIFAR10_testing_plot_centroid_distance_bars.png}
\end{figure}

% is a bar chart representing the mean softmax distances to class centroid for all correct (green) and all incorrect (red) classifications from the ViT model trained on CIFAR-10 data. 

% The softmax distribution bar charts provide a view of the model's confidence and uncertainty in its predictions. The distinct patterns observed for correct and incorrect classifications offer valuable information about the model's decision-making process.

Figures \ref{fig:CIFAR10_training_plot_centroid_distance_bars.png} and \ref{fig:CIFAR10_testing_plot_centroid_distance_bars.png} bar charts show the average softmax distributions for correct (green) and incorrect digit predictions in both the testing and training CIFAR-10 datasets. The softmax values are presented on a logarithmic scale, emphasizing the relative differences between the predicted probabilities for each digit class.

For correctly classified instances, the average softmax value corresponding to the true digit class is significantly higher compared to the softmax values of the other digit classes. This observation holds true across all digit classes in both the testing and training datasets. The pronounced difference in magnitudes indicates that the model assigns a high level of confidence to the correct predictions, with the predicted probability for the true class being orders of magnitude larger than the probabilities assigned to the other classes.

In contrast, for incorrectly classified instances, the average softmax values exhibit a more even distribution across the digit classes. While the softmax value for the predicted class is still relatively high, the softmax values for the other classes are notably closer in magnitude, as evident from the shorter bars on the logarithmic scale. This suggests that when the model makes an incorrect prediction, it assigns more substantial probabilities to multiple classes, indicating a higher level of uncertainty or confusion in the decision-making process.

Comparing the testing and training datasets, we observe similar patterns in the softmax distributions for both correct and incorrect predictions. The consistency of these patterns suggests that the model generalises well from the training data to unseen testing data. However, it is worth noting that the average softmax values for incorrect predictions in the testing dataset appear to be slightly more evenly distributed compared to those in the training dataset. 

The analysis of these softmax distributions may be taken as an insight into the model's decision-making process. The difference in the softmax values between correct and incorrect predictions highlights the model's ability to discriminate between classes when it makes accurate predictions. On the other hand, the more evenly distributed softmax values for incorrect predictions suggest that the model struggles to make clear distinctions between classes in those cases, assigning considerable probabilities to multiple digits.

Further investigation into the characteristics of the incorrectly classified instances could yield additional insights. Examining the specific examples where the model assigns high probabilities to multiple classes may reveal common patterns or features that contribute to the model's confusion. Such analysis could guide efforts to improve the model's performance, such as refining the training data or adjusting the model architecture.

% Figure generated by function call:
% boxplots_side_by_side_x2(d2c_train_correct, d2c_train_incorrect, d2c_test_correct_train_centroids, d2c_test_incorrect_train_centroids, False, True, title1="Training Data Boxplots of Softmax Distances to Training Centroids", title2="Testing Data Boxplots of Softmax Distances to Training Centroids")
\begin{figure*}[h]
    \centering
    \includegraphics[width=0.99\textwidth]{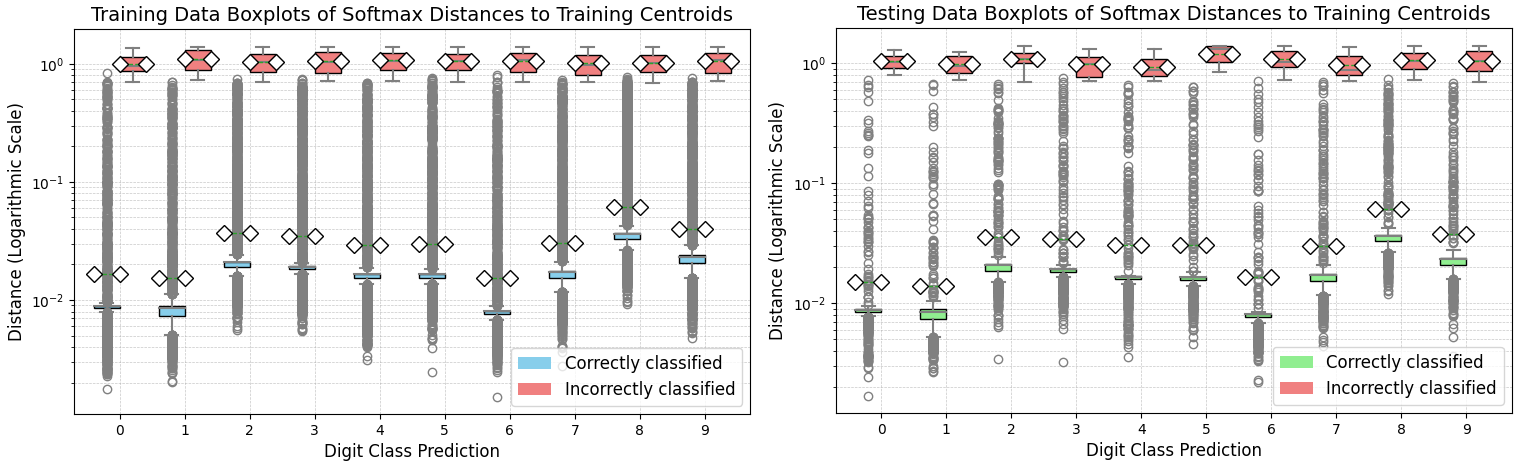}   \captionsetup{justification=raggedright,singlelinecheck=false}
    \caption{Distribution of Distances to Centroids for Correctly and Incorrectly Classified Instances in Training and Testing MNIST Data, where training data is on the left and testing data is displayed on the right. Distances are shown on a logarithmic scale. Note, centroids are for the correctly classified training examples, for both training and testing dataset.}
    \label{fig:boxplots_side_by_side_x2_training_centroids}
\end{figure*}

\subsection{Algorithms}
\label{apppendix:algorithms}

\begin{algorithm}
\caption{K-Means Centroid Initialisation from Softmax Outputs}
\label{alg:k-means-centroid-init} 
\begin{algorithmic}[1]
\Require{$correct\_preds$: array of shape $(n, 12)$, where $n$ is the number of correct predictions}
\Ensure{$centroids$: array of shape $(10, 10)$, initialised centroids for each digit class}

\State $probs\_dist \gets corrects\_preds[:, :10]$ \Comment{Extract probability distribution for each digit}
\State $centroids \gets \text{zeros}((10, 10))$ \Comment{Initialise centroids array}

\For{$digit \gets 0$ to $9$}
\State $indices \gets \text{where}(\text{argmax}(probs\_dist, \text{axis}=1) == digit)[0]$ \Comment{Find indices of rows where digit has highest probability}
\State $centroid \gets \text{mean}(probs\_dist[indices], \text{axis}=0)$ \Comment{Compute mean probability distribution for selected rows}
\State $centroids[digit] \gets centroid$ \Comment{Assign centroid to corresponding row in centroids array}
\EndFor

\State \textbf{return} $centroids$
\end{algorithmic}
\end{algorithm}

\begin{algorithm}
\caption{Find Minimum Softmax Distances to Centroids for Incorrectly Predicted Digits (Threshold)}
\label{alg:min_distance} 
\begin{algorithmic}[1]
\Procedure{FindMinDistances}{$data$}
    \State $labels \gets [0, 1, 2, 3, 4, 5, 6, 7, 8, 9]$
    \State $thresh \gets \text{empty array of shape } (10, 2)$
    \For{$i \gets 0 \text{ to } 9$}
        \State $label \gets labels[i]$
        \State $min\_dist \gets \min(data[data[:, 1] == label, 0])$
        \State $thresh[i, 0] \gets min\_dist$
        \State $thresh[i, 1] \gets label$
    \EndFor
    \State \textbf{return} $thresh$
\EndProcedure
\end{algorithmic}
\end{algorithm}
